# Supplementary material for: Probing spin correlations in a Bose-Einstein condensate near the single atom level
Source: arXiv:2004.09003 ancillary file (2020-07-11)
Supplement: Supplementary file 1 [file ProbingSpinCorr_SM.pdf]

# Supplemental Material:

## Probing spin correlations in a Bose–Einstein condensate near the single atom level

An Qu, Bertrand Evrard, Jean Dalibard and Fabrice Gerbier  
*Laboratoire Kastler Brossel, Collège de France, CNRS,  
 ENS-PSL Research University, Sorbonne Université,  
 11 Place Marcelin Berthelot, 75005 Paris, France*  
 (Dated: June 25, 2020)

### I. DETAILS OF THE EXPERIMENTAL SETUP

#### A. Details of the experimental preparation

We prepare a Bose–Einstein condensate (BEC) of sodium atoms in a crossed dipole trap, and perform fluorescence imaging after a time-of-flight expansion in a magnetic field gradient. In detail, we suddenly (in less than  $100\,\mu\text{s}$ ) switch off the optical trap. This marks the beginning of the expansion  $t_0 = 0$ . Before and during the expansion, the atoms experience a horizontal bias magnetic field around 2 G and an additional magnetic field gradient switched on at  $t_0$ . The gradient ramps up to its peak value (around 10 G/cm) in approximately 3 ms. The atoms fall under gravity and also separate horizontally due to the Stern–Gerlach (SG) force. We gradually switch off the magnetic gradient and bias field until  $t_2 = 10\,\text{ms}$ . At  $t_3 = 18\,\text{ms}$ , we finally switch on the optical molasses (OM) for a duration  $t_{\text{mol}}$ . The separation between the  $m = 0$  and the  $m = \pm 1$  components is  $d_{\text{SG}} \sim 1.32\,\text{mm}$ .

The timing of this sequence results from a trade-off between several experimental constraints. Since the waist ( $1/e^2$  radius) of the OM beams is limited ( $\sim 1\,\text{cm}$ ), atoms eventually move out of the OM area. We limit the total duration of the sequence to less than 30 ms to maintain the atoms near the beam center during the whole OM duration. In addition, the strength of the SG gradient cannot be increased or decreased arbitrarily fast. Eddy currents developing in the apparatus when the magnetic fields are switched off are detrimental to the operation of the OM. The empirically determined delay between  $t_2$  and  $t_3$  is inserted to ensure that the magnetic fields have decayed to a sufficiently low value.

#### B. Optical molasses

The OM forms at the intersection of three mutually orthogonal laser beam pairs. These beams induce resonant fluorescence on the  $F = 2 \rightarrow F' = 3$  transition of the  $D_2$  line of the Sodium atom (resonant wavelength  $\lambda_0 \approx 589.2\,\text{nm}$ ) and simultaneously cool the atoms in three dimensions. A repumper beam resonant with  $F = 2 \rightarrow F' = 2$  is superimposed with each OM beam to maintain cycling on the main cooling transition. We use the same optical setup as for the magneto-optical trap used in the beginning of the cooling sequence leading to

the production of the BEC.

We operate the OM with an intensity  $I = 3.1\,\text{mW}/\text{cm}^2$  per beam. We optimize the detuning  $\delta_{\text{mol}}/(2\pi) \approx -9.9\,\text{MHz}$  to limit the cloud expansion during the OM phase while keeping a sizable fluorescence signal (see below for a detailed analysis of both aspects).

#### C. Background light

Besides fluorescence photons, the imaging system also collect spurious (“background”) signal from various sources. The dominant part of this background light comes from scattering of the OM beams from various reflective parts of the apparatus, including the vacuum chamber walls and viewports. The vacuum chamber also hosts a background sodium gas at room temperature and very low pressure ( $< 10^{-11}\,\text{mbar}$ ). The low-energy tail of the atomic distribution can be captured in the OM and contributes a spurious fluorescence signal. Using “empty” images acquired without loading the optical trap, we measure that the total background light amounts to the total fluorescence from a cloud of about one thousand ultracold atoms. Fortunately, the spatial distribution of this background light is very broad and easily distinguished from the fluorescence signal of interest. Image processing discussed in Section II C allows us to essentially cancel this contribution.

#### D. Estimation of the atomic fluorescence

We simplify the level structure of a sodium atom and treat it as a two-level system with the same electric dipole as the  $F = 2, m_F = +2 \rightarrow F' = 3, m_{F'} = +3$  transition. We also assume that the contribution from each beam can be added independently for simplicity. The mean fluorescence rate per atom is then

$$\Gamma_{\text{sp}} = \frac{\Gamma}{2} \frac{s_0}{1 + (\frac{2\delta_{\text{mol}}}{\Gamma})^2 + s_0} \approx 1.2 \times 10^7 \text{ photons/s}, \quad (1)$$

with the natural linewidth  $\Gamma/(2\pi) \approx 10.0\,\text{MHz}$ , the saturation intensity for a  $\sigma^+$  transition  $I_{\text{sat}} \approx 6.2\,\text{mW}/\text{cm}^2$ , and the total saturation parameter  $s_0 = 6I/I_{\text{sat}} \approx 3.0$ . In principle this independent beam approximation should only hold for very weak saturation levels, however it provides a relevant estimation of the expected signal in our setup.

## II. ANALYSIS OF FLUORESCENCE SIGNAL

### A. Detected photon flux

The fluorescence signal recorded on the camera results from an integration of the collected photon flux over the entire duration  $t_{\text{mol}}$  of the OM phase. In our analysis, we assume that the three Zeeman components are sufficiently well separated, so that a given point  $\mathbf{r} = (x, y)$  in region  $A_m$  of the image can be associated unambiguously to a single component  $m$  (see below). We write the fluorescence profile recorded by the camera in  $A_m$  as

$$I_{\text{flu},m}(\mathbf{r}, t_{\text{mol}}) = \int_0^{t_{\text{mol}}} dt \bar{\phi}_m \rho_m(\mathbf{r}, t). \quad (2)$$

To lighten notations, we use continuous coordinates  $\mathbf{r}$  to indicate the signal on each pixel of the camera, being understood that we are dealing with signals integrated over each pixel area. The instantaneous atomic distribution  $\rho_m(\mathbf{r}, t)$  is normalized such that  $\sum_{\mathbf{r} \in A_m} \rho_m(\mathbf{r}, t) = N_m$ .

The quantity  $\bar{\phi}_m$  is the detected photon flux per atom in the Zeeman component  $m$  collected in region  $A_m$  (see Fig. 2 of the main article). Generally, this flux is proportional to  $\Gamma_{\text{sp}}$ . The proportionality factor depends on many experimental details, such as the solid angle of collection of the front-end microscope objective, the camera efficiency, and the optical losses along the imaging path. A best-case estimate for this factor is  $0.73 \times \text{NA}^2/4 \approx 0.016$ , where the first number is the measured efficiency of the CCD camera and the second is a geometric collection factor for the numerical aperture  $\text{NA} \simeq 0.30$  [1]. This gives an upper bound for the detected photon flux per atom

$$\bar{\phi}_m^{(\text{th})} \lesssim 195 \text{ photons/ms}. \quad (3)$$

Integrating  $I_{\text{flu},m}$  over the ROI  $A_m$ , we obtain the number of detected fluorescence photons,

$$\mathcal{S}_m^{(\text{flu})} = \sum_{\mathbf{r} \in A_m} I_{\text{flu},m}(\mathbf{r}, t_{\text{mol}}) = N_m \bar{\phi}_m t_{\text{mol}}. \quad (4)$$

In the following, we discuss the various steps leading from the recorded fluorescence profile to the final estimation of the atomic population  $N_m$ . We explain how the parameters  $t_{\text{mol}}$  and the optimized region of integration  $A'_m$  are chosen. We describe image processing techniques essential to reject the average contribution of background light and to calibrate the fluxes  $\bar{\phi}_m$ . We finally discuss the noise and the sensitivity of the measurement of the Zeeman populations.

### B. Spatial diffusion in the optical molasses

We first address the spatial distribution of the fluorescence signal. In the remainder of this Section, we consider

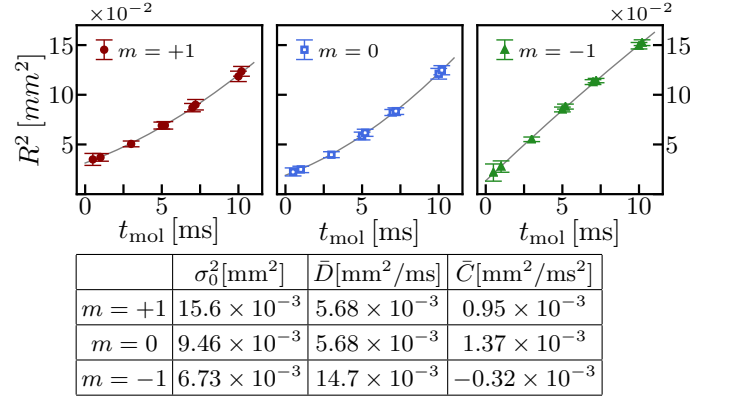

FIG. 1. Spatial variances  $R^2(t_{\text{mol}})$  of the fluorescence distribution for each Zeeman component  $m = +1, 0, -1$ . The color points with error bars are data. A fit to the data (grey curves) using Eq. (6) provides the arithmetic average  $\bar{D}$  and  $\bar{V}$  of the diffusion coefficients and of the velocity. The fitted values are given in the table.

one particular component and drop the Zeeman index  $m$  for simplicity.

The atomic profile  $\rho$  is not stationary due to spatial diffusion in the OM [2]. We model the density profile  $\rho(\mathbf{r}, t)$  by an isotropic Gaussian distribution centered at  $\mathbf{r}_0 = (x_0, y_0)$  and with a standard deviation  $\sigma_i(t)^2 = \sigma_0^2 + 2D_i t + C_i t^2$  along directions  $i = x, y$ . Here,  $\sigma_0$  represents the size of the initial distribution,  $D_i$  is the diffusion coefficient and  $C_i$  accounts for a ballistic component in the expansion due to inhomogeneous forces. The latter would not occur in an ideal OM, but may arise due to experimental imperfections such as a residual magnetic field or a small imbalance between the OM beams.

The variance  $R^2$  of the fluorescence distribution is

$$R^2(t_{\text{mol}}) = \frac{1}{\mathcal{S}_m^{(\text{flu})}} \sum_{\mathbf{r} \in A_m} (\mathbf{r} - \mathbf{r}_0)^2 I_{\text{flu}}(\mathbf{r}, t_{\text{mol}}). \quad (5)$$

Using Eq. (2), this can be rewritten as

$$R^2 = \frac{1}{t_{\text{mol}}} \int_0^{t_{\text{mol}}} dt \sigma^2(t) = 2\sigma_0^2 + \bar{D} t_{\text{mol}} + \frac{\bar{C} t_{\text{mol}}^2}{3} \quad (6)$$

with  $\bar{D} = D_x + D_y$  and  $\bar{C} = C_x + C_y$ .

We show in Fig. 1 the measured spatial variances  $R^2$  for each spin component. For the typical OM time  $t_{\text{mol}} = 5 \text{ ms}$  used in our measurements, the maximum standard deviation of the clouds is  $\approx 0.27 \text{ mm}$ , much smaller than the separation distance  $d_{\text{SG}} \approx 1.3 \text{ mm}$ .

The rate of false assignments, *i.e.* the probability to find an atom in Zeeman state  $m$  in the wrong region  $A'_m$ , can be estimated from the Gaussian model and the measured diffusion coefficients. For the raw square regions of interest (ROIs)  $A_m$  shown in Fig. 1 of the main paper, the probability to find a  $m = +1$  atom in the  $m = 0$  region  $A_0$  is less than 1 %. Using the optimized ROIs  $A'_m$  (see the main article and Section II C) further reduces the probability to less than 0.1 %.

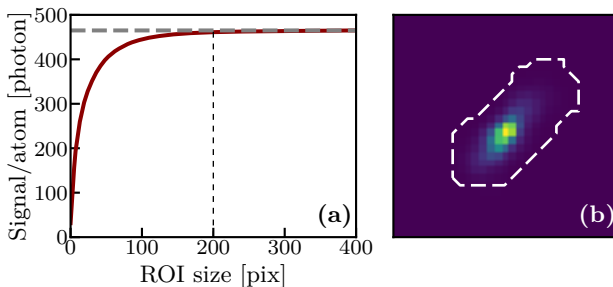

FIG. 2. **(a)**. The red solid line shows the average fluorescence flux versus the ROI size for  $t_{\text{mol}} = 5$  ms. The horizontal grey line is the total signal collected in the squared ROI  $A_m$ . The vertical line is the cutoff size of the optimized ROI  $A'_m$ . **(b)**. Optimized ROI  $A'_0$  for the cut-off threshold 99%.

### C. Image processing

We process fluorescence images in two successive steps.

*a. Choice of optimized ROI  $A'_m$ .* For each “raw” ROI  $A_m$ , we order the pixels by brightness in decreasing order. We then decide on a cut-off level and reject all pixels below that level. We choose the cutoff so that the signal after selection is 99% of the total signal, which defines  $A'_m$ . This procedure excludes about 1/2 of the pixels from the original raw ROI  $A_m$ . We show in Fig. 2 (a) the measured photon flux for the optimized ROI for various cutoff levels. The flux inside  $A'_m$  reaches the threshold at a size of 200 pixels. This behavior gives another confirmation that the support of the spatial distribution of fluorescence is indeed much smaller than the size of the integration region  $A_m$ . We conclude that the discarded pixels contain little information about the atoms. Effectively, we discard pixels which are mostly collecting background light and select pixels which are mostly collecting atomic fluorescence.

*b. Background subtraction:* In a second step, we apply a normalization algorithm to remove the mean signal due to background light, effectively cancelling it from each image. We use an algorithm known as “eigenface method” in the image processing literature, and introduced to the field of cold atoms in [3]. Below, we use the term “Best reference picture” (BRP) algorithm to refer to this method. The BRP method uses all pixels outside of the ROIs  $A_m$  to determine the distribution of background light inside the ROIs. The algorithm uses a set of “empty” images (*i.e.* without atoms) to determine the mean distribution of background light. For a given image (with atoms), the BRP algorithm seeks for the best linear combination of the images in the “empty” set that reproduces the observed signal. This determines the background that we subsequently subtract from the actual image. Because of the broad and smooth spatial distribution of background light, the BRP algorithm is very efficient at suppressing the average background contribution, as illustrated in Fig. 3) and discussed in

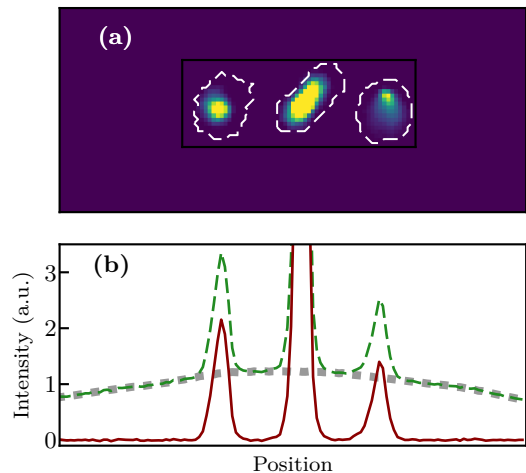

FIG. 3. Illustration of the BRP algorithm on a typical image. **(a)** Raw image to be processed. The rectangle zone and the dashed contours are respectively ROIs  $A_m$  and  $A'_m$ . The hatched zone is used for the BRP algorithm. **(b)** The green dashed profile comes from the raw image with atoms. The three peaks correspond to three clouds, but the signal is mixed with stray light. The red solid profile represents the fluorescence signal after removing the stray light by the BRP algorithm. The background stray light profile obtained by the BRP algorithm is shown by the large dotted grey profile. It is calculated from a linear combination of the series of “empty” images.

the next Section.

### D. Estimation of Zeeman state populations

We now turn to the estimation of the total number of atoms contributing to the photon signal collected in region  $A_m$ . The contribution from background light (integrated photon flux  $\bar{\phi}_{\text{bg}}$  in  $A'_m$ ) is *a priori* independent of the atom number  $N_m$  to be determined. The total integrated photon count over the optimized ROI  $A'_m$  can be written as

$$\bar{S}_m = (N_m \bar{\phi}_m + \bar{\phi}_{\text{bg}}) t_{\text{mol}}. \quad (7)$$

Using the BRP algorithm allows us to essentially suppress the second contribution. We tested the algorithm on a set of empty images. Without processing, we typically find  $\bar{\phi}_{\text{bg}} \approx 8.7 \times 10^4$  photons/ms (the equivalent of the fluorescence signal from  $\sim 1000$  atoms, see below). Applying the BRP algorithm, we find that the contributions are reduced to very small levels compatible with zero with an uncertainty of  $\sim 4$  photons/ms (much less than the signal of a single atom, see below). We finally obtain an (almost) unbiased estimator of the true Zeeman population  $N_m$  from

$$\mathcal{N}_m = \frac{\bar{S}_m}{\bar{\phi}_m t_{\text{mol}}}, \quad (8)$$

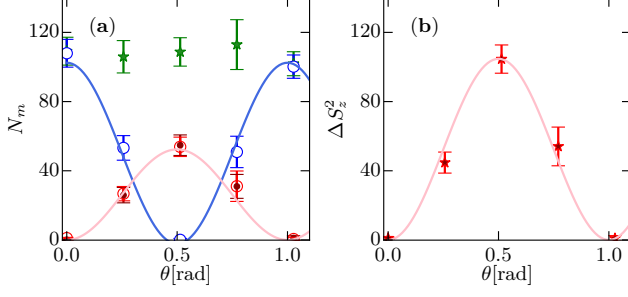

FIG. 4. **a** Evolution of the populations  $N_0$  (blue circles),  $N_{+1}$  (red circles) and  $N_{-1}$  (red dots) over a Rabi oscillation. The fluorescence fluxes are determined as to make the total atom number  $N$  (green stars) constant and equal to the value measured using absorption imaging. Alternatively, one can use the evolution of the partition noise  $\Delta S_z^2$  (**b**, red stars) to calibrate all fluorescence fluxes without relying on absorption imaging. The solid lines are fits to the data.

with  $\bar{S}_m$  the sum over the processed images.

### E. Calibration of fluorescence flux

So far, the photon fluxes per atom  $\bar{\phi}_m$  are unknown. We calibrate them against absorption imaging, which is itself calibrated by comparing the measured spatial atomic distribution with the one calculated from the Gross–Pitaevskii equation. We first measure the mean atom number  $\bar{N}_0^{\text{abs}}$  for a BEC polarized in the  $m = 0$  Zeeman component using absorption imaging, and the total fluorescence signal  $\bar{S}_0$  in the same conditions. We get

$$\bar{\phi}_0 = \frac{\bar{S}_0}{\bar{N}_0^{\text{abs}} t_{\text{mol}}} \approx 93 \pm 3 \text{ photons/at/ms.} \quad (9)$$

Second, we calibrate  $\bar{\phi}_{\pm 1}/\bar{\phi}_0$ . We start from the same initial cloud with all atoms in  $m = 0$  and apply a spin rotation of angle  $\theta$  along  $y$ . The Zeeman populations evolve as

$$N_0(\theta) = N \cos^2 \theta, \quad (10)$$

$$N_{\pm 1}(\theta) = \frac{N}{2} \sin^2 \theta. \quad (11)$$

We measure the fluorescence signal for different values of  $\theta$ , and find  $\bar{\phi}_{\pm 1}$  as the values that make the total atom number independent of  $\theta$ . The results are shown in figure 4 **a**. This procedure gives

$$\bar{\phi}_{+1} = 89 \pm 3 \text{ photons/at/ms,} \quad (12)$$

$$\bar{\phi}_{-1} = 86 \pm 3 \text{ photons/at/ms.} \quad (13)$$

The measured fluxes are almost independent of the Zeeman state and their value is about half of the estimation in Eq. (3). The difference presumably comes from

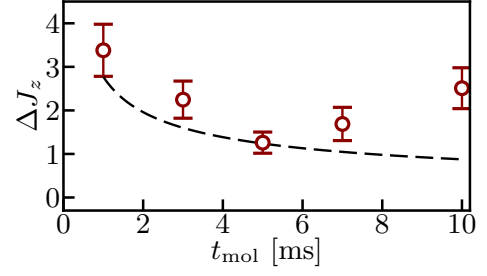

FIG. 5. Measured standard deviation (red circles) of  $J_z$  as a function of  $t_{\text{mol}}$ . The dashed black line is the estimated best achievable number resolution given by Eq. (15).

the multi-level structure of the Sodium atom, leading to optical pumping effects that lower the absorption and emission cross-sections.

An analysis of the partition noise during a Rabi oscillation [4], shown in figure 4 **b**, allows one to check the previous calibration without relying on absorption imaging. Indeed, the variance of  $S_z = N_{+1} - N_{-1}$  evolves over the rotation as

$$\Delta S_z^2(\theta) = N_{+1} + N_{-1}. \quad (14)$$

The equation, together with Eqs. (10, 11), constitutes a sufficient set to determine the three fluxes  $\bar{\phi}_m$  and the total atom number  $N$ . This alternative method gives identical results within error bars, and leads to a similar uncertainty.

### F. Imaging noise and detection sensitivity

We now discuss the noise level associated with the fluorescence signal. We have identified three possibly relevant sources of noise, namely the shot noise of fluorescence and background light, and the electronic noise of the camera.

We first discuss the contribution of the electronic noise  $\eta_{\text{cam}} A'_m$  and show that it can be essentially eliminated using hardware binning. In our imaging procedure, we bin  $B^2$  adjacent pixels, defining thus a “macro-pixel”, and we process them together in the readout stage of the camera. We have checked that the camera noise is uniform across the entire CCD, with a standard deviation per macro-pixel  $\sqrt{\eta_{\text{cam}}} \approx 3.6 + 0.36B$  photons. For our choice of  $B = 8$  and  $A'_m = 200$  macro-pixels, we find that the camera noise corresponds to 90 counts, *i.e.* equivalent to the signal from  $\approx 0.2$  atom for  $t_{\text{mol}} = 5$  ms and negligible compared to the photonic noise. We thus neglect this contribution from now on.

The atom number estimator after background subtraction  $\mathcal{N}_m$  is a random variable. Its distribution reflects the combined distributions of fluorescence and background photons, which are *a priori* independent Poisson pro-

cesses. The variance of  $\mathcal{N}_m$  is thus given by

$$\Delta \mathcal{N}_m^2 \approx \frac{N_m}{\bar{\phi}_m t_{\text{mol}}} + \frac{\bar{\phi}_{m,\text{bg}}}{\bar{\phi}_m^2 t_{\text{mol}}}. \quad (15)$$

This expression is useful for the optimization of the OM duration  $t_{\text{mol}}$ . The first contribution in the right-hand side is clearly a decreasing function of  $t_{\text{mol}}$ . The behavior of the second contribution is more subtle, because there is actually an implicit dependence on  $t_{\text{mol}}$  hidden in  $\bar{\phi}_{m,\text{bg}}$ . Since the background light signal is spatially very broad, we expect the mean flux (and thus the associated shot noise) to scale as the integration area,  $\bar{\phi}_{m,\text{bg}} \propto A'_m$ . Since this area is optimized to track the cloud radius, it scales with the cloud area  $D_m t_{\text{mol}}$ , with  $D_m$  the spatial diffusion coefficient determined in § II B. As a result, we expect that  $\bar{\phi}_{m,\text{bg}}$  also scales as  $t_{\text{mol}}$ . In this situation, the contribution of the background light shot noise [second term in Eq. (15)] is approximately independent of  $t_{\text{mol}}$ .

In order to choose the optimal value of  $t_{\text{mol}}$ , one must also consider atom losses during the molasses phase, which create a bias of the detected atom number. The most relevant processes are the inelastic collisions assisted by the quasi-resonant light of the molasses beams, and we expect the corresponding losses to increase with  $t_{\text{mol}}$ . The combination of the two contributions of Eq. (15) and of the atom losses results in an optimal value of  $t_{\text{mol}}$ . This is illustrated in Fig. 5 where we plot the standard deviation  $\Delta J_z^2 = (\Delta \mathcal{N}_{+1}^2 + \Delta \mathcal{N}_{-1}^2)/4$ . For a long OM duration  $t_{\text{mol}}$ , we expect the variance of  $\mathcal{N}_m$  to increase with the mean number of lost atoms and thus also with  $t_{\text{mol}}$ . This is indeed observed in Fig. 5, with a minimal value around  $t_{\text{mol}} = 5$  ms. We therefore choose  $t_{\text{mol}} = 5$  ms in all measurements discussed in the article to minimize the detection noise.

### G. Correction of systematic errors on $J_z$

The uncertainty of absorption imaging as well as its spatial inhomogeneity are at the level of a few percent. This leads to a systematic error on the absolute values of the individual Zeeman populations  $N_m$ . Indeed  $\bar{\phi}_m^{(\text{true})} = \bar{\phi}_m(1 + \epsilon_m)$ , where the  $\bar{\phi}_m^{(\text{true})}$  are the true values of the photon flux and  $\bar{\phi}_m$  the values inferred from the comparison between fluorescence and absorption imaging [cf. Eqs (12-13)]. This issue may be problematic when we estimate the angular momentum along  $z$ ,

$$\bar{J}_z = \frac{1}{2} \left( \frac{\bar{S}_{+1}}{\bar{\phi}_{+1}} - \frac{\bar{S}_{-1}}{\bar{\phi}_{-1}} \right) \approx (1 + \bar{\epsilon}) \bar{J}_z + \frac{\epsilon_d}{2} \bar{N}_p, \quad (16)$$

where we have expanded the right hand side to lowest order in  $\epsilon_{\pm 1}$  and introduced the mean and the difference of the  $\epsilon_m$ 's:

$$\bar{\epsilon} = \frac{1}{2} (\epsilon_+ + \epsilon_-), \quad \epsilon_d = \epsilon_+ - \epsilon_-. \quad (17)$$

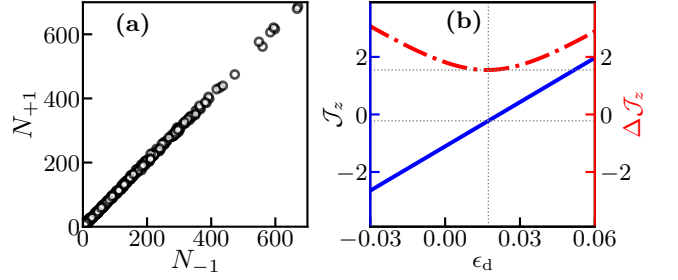

FIG. 6. (a) Measured value of  $N_{+1}$  as a function of  $N_{-1}$  for the TMSV state at  $t_{\text{osc}} = 150$  ms. The atom numbers are converted from photon signal using the average fluorescent fluxes  $\bar{\phi}_m$ . A linear fit to these data gives the slope 1.021. (b)  $\Delta \bar{J}_z$  and  $\bar{J}_z$  as a function of the correction factor. The closeness of the minimum of  $\Delta \bar{J}_z$  ( $\epsilon_d = 0.017$ ) and of the zero point of  $\bar{J}_z$  ( $\epsilon_d = 0.021$ ) is a check of the validity of our modelling of systematic errors.

Here  $\bar{J}_z$  is the measured value affected by systematic errors and  $J_z, N_p$  are the true values.

In practice, for the TMSV state of interest in this work, only the term  $\epsilon_d \bar{N}_p/2$  is significant in (16), because it injects the contribution of a large number ( $\bar{N}_p$ ) into a quantity that is a priori expected to be very small ( $\bar{J}_z$ ). Therefore we take  $\epsilon_d$  as the relevant correction factor and we arbitrarily set the other independent factor  $\bar{\epsilon}$  to zero. This only entails an error of 1 – 2 % on the number of pairs  $N_p$ , which has no impact on our results.

Fig. 6(a) demonstrates the expected linear relation between  $N_{\pm 1}$  for the TMSV state produced at  $t_{\text{osc}} = 150$  ms, measured without correcting for the calibration factors. A linear fit to the data provides the slope  $1.021 \approx 1 + \epsilon_d$ , hence  $\epsilon_d = 0.021$ . The same data are used for the blue line in Fig. 6(b), where we plot  $\bar{J}_z$  as a function of  $\epsilon_d$  and we find it to vanish for  $\epsilon_d = 0.021$ . The slope of this line  $\sim 51$  is in good agreement with the prediction (16), with  $\bar{N}_p = 105$  for the TMSV state at  $t_{\text{osc}} = 150$  ms.

Even for a perfectly balanced sample with  $J_z = 0$  but a fluctuating  $N_p$  (as for the TMSV state), small systematic errors  $\epsilon_{\pm 1}$  result not only in a non-zero detected  $\bar{J}_z$ , but also in an increase of the detected variance  $\Delta \bar{J}_z$ . We confirm this prediction by plotting in Fig. 6(b) the variation of  $\Delta \bar{J}_z$  as a function of the correction factor  $\epsilon_d$  (red dashed line). We check that  $\Delta \bar{J}_z$  is minimal around the same value of  $\epsilon_d$  as the one inferred from the variation of  $\bar{J}_z$ , which is a good sanity check of our modelling.

Here we used a TMSV state obtained at  $t_{\text{osc}} = 150$  ms ( $\bar{N}_p \sim 100$ ) to evaluate the correcting factor  $\epsilon_d$ . We have checked that the value of  $\epsilon_d$  – and thus the squeezing factor obtained in the article – is unchanged (within error bars) if we use a TMSV at  $t_{\text{osc}} = 50$  ms ( $\bar{N}_p \sim 5.2$ ) and  $t_{\text{osc}} = 100$  ms ( $\bar{N}_p \sim 23$ ) for the calibration described above.

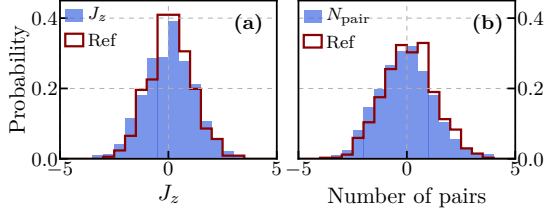

FIG. 7. Blue histograms: characterization of the initial state. (a) Distribution of  $J_z = (N_{+1} - N_{-1})/2$ . (b) Distribution of the number of pairs  $N_p = (N_{+1} + N_{-1})/2$ . The red lines are reference measurements taken on empty images.

### III. CHARACTERIZATION OF A FOCK STATE

Fig. 7 shows the characterization of the initial state in terms of probability distributions for  $J_z$  and  $N_p$ , obtained from 1026 runs of the experiment. We recall that for this initial state, we aim at having all atoms in the state  $m = 0$ . Therefore for comparison, we show on the same figure the histograms obtained with “empty” reference images, taken using the same experimental sequence, but without loading any atom (627 runs). Since the two distributions, with or without atoms, do not show any statistically significant difference, we infer that the  $m = \pm 1$  counts for our initial state can be accounted for by detection noise only (mean pair number  $N_p = 0.112 \pm 0.046$  without atoms and  $N_p = -0.050 \pm 0.040$  with atoms).

### IV. NON-SEPARABILITY CRITERION

Consider an assembly of  $N$  particles with pseudo-spin  $j = 1/2$ , described by the collective spin operators  $\hat{\mathbf{J}} = \sum_{i=1}^N \hat{\mathbf{j}}_i$ . If the  $N$ -spin state is separable, the following inequality holds [5]:

$$\langle \hat{J}_x^2 \rangle + \langle \hat{J}_y^2 \rangle - \frac{N}{2} \leq (N-1) (\Delta J_z)^2. \quad (18)$$

Therefore one can define the *entanglement parameter* (or *generalized spin-squeezing parameter*) [6]

$$\xi_{\text{os}}^2 = \frac{(N-1) (\Delta J_z)^2}{\langle \hat{J}_x^2 \rangle + \langle \hat{J}_y^2 \rangle - \frac{N}{2}} \quad (19)$$

and infer from (18) that any result  $\xi_{\text{os}}^2 < 1$  signals a non-separable state. This indicator was used in [7] to detect entanglement of Dicke states. The Hilbert space of the  $N$ -spin system has a dimension  $2^N$ . If the  $N$  spins are prepared in a fully symmetric state, the size of the Hilbert space is only  $N+1$  since it corresponds to that of an angular momentum  $J = N/2$ . In this completely symmetric subspace  $\hat{J}_x^2 + \hat{J}_y^2 + \hat{J}_z^2 = N(N+2)/4$  and the inequality (18) can be written [8, 9]

$$\frac{N^2}{4} - \langle \hat{J}_z^2 \rangle \leq (N-1) (\Delta J_z)^2. \quad (20)$$

In our experiment, we assume that the state of the  $N_{\text{tot}}$  spin-1 atoms is described within the single spatial mode approximation. The spin state of the  $N_{\text{tot}}$  atoms must therefore be fully symmetric with respect to exchange of any two particles and it can be written using the formalism of second quantization:

$$|\Psi\rangle = \sum_{N=0}^{N_{\text{tot}}} C_N \frac{(\hat{a}_0^\dagger)^{N_{\text{tot}}-N}}{\sqrt{(N_{\text{tot}}-N)!}} \mathcal{F}_N \left( \hat{a}_1^\dagger, \hat{a}_{-1}^\dagger \right) |\text{vac}\rangle \quad (21)$$

(or as a statistical mixture of such states). Here  $\hat{a}_m^\dagger$  creates a particle in the Zeeman state  $m$  and in the spatial mode of the condensate, and the state

$$|\Phi_N\rangle \equiv \mathcal{F}_N \left( \hat{a}_1^\dagger, \hat{a}_{-1}^\dagger \right) |\text{vac}\rangle \quad (22)$$

describes a normalized, fully symmetric state of  $N$  particles in the two Zeeman states  $m = \pm 1$ , which can be viewed as a collection of  $N$  pseudo-spins 1/2 particles. The quantity  $|C_N|^2$  gives the probability to have  $N$  particles in  $m = \pm 1$  and  $N_{\text{tot}} - N$  particles in  $m = 0$ . For any measurement of a quantity  $\mathcal{O}$  dealing only with the  $m = \pm 1$  Zeeman states, the expectation value is the weighted average:

$$\langle \Psi | \hat{\mathcal{O}} | \Psi \rangle = \sum_N |C_N|^2 \langle \Phi_N | \hat{\mathcal{O}} | \Phi_N \rangle. \quad (23)$$

Suppose now that each  $|\Phi_N\rangle$  (which is by construction fully symmetric) is also separable. Then (20) applies to each of them and it also applies to their average over  $N$  with the weights  $|C_N|^2$ . Since one can divide (20) by any power of  $N$  before averaging, this allows one to derive a set of inequalities that must be satisfied for separable states, such as:

$$\xi_{\text{os},1}^2 \equiv \frac{\langle (N-1) (\Delta J_z)^2 | \Phi_N \rangle}{\frac{\langle N^2 \rangle}{4} - \langle \hat{J}_z^2 \rangle} > 1 \quad (24)$$

and

$$\xi_{\text{os},2}^2 \equiv \frac{\langle (1 - \frac{1}{N}) (\Delta J_z)^2 | \Phi_N \rangle}{\frac{\langle N \rangle}{4} - \langle \frac{\hat{J}_z^2}{N} \rangle} > 1. \quad (25)$$

We used the generalized spin-squeezing parameter  $\xi_{\text{os},2}$  in the main text, with the simplification valid for the large  $N = 2N_p$  values that are relevant in our experiment:

$$\xi_{\text{os},2}^2 \approx 4 \frac{\langle (\Delta J_z)^2 \rangle}{\langle N \rangle}, \quad (26)$$

with the  $N$ -average taken over bins of width  $\Delta N = 100$  (i.e.  $\Delta N_p = 50$ ). This parameter was also used in [10–12] to detect number-squeezing in spinor BECs.

### V. INTERFEROMETRIC SENSITIVITY OF A TWO-MODE SQUEEZED VACUUM STATE INCLUDING DETECTION ERRORS

Two-mode Mach-Zehnder interferometric measurements with twin Fock states or two-mode squeezed vac-

uum (TMSV) states have been studied in detail in the context of quantum optics [13–15]. Each mode (here  $m = \pm 1$ ) is injected in one of the two input ports, and one measures the difference between the intensities of the two output ports. The signal of the interferometer is characterized by the operator  $\hat{J}'_z = \cos \theta \hat{J}_z + \sin \theta \hat{J}_x$  with  $\theta$  the phase shift between the two paths and  $\hat{\mathbf{J}}$  the pseudo-spin operator describing the input [15].

For input twin Fock states or TMSV states, the output of the interferometer is always balanced on average,  $\langle J'_z \rangle = 0$ . The phase information is contained in the variance  $\langle J'^2_z \rangle$ . The corresponding phase sensitivity is, taking  $S \equiv J'^2_z$  as the observable,

$$\Delta\theta = \frac{\Delta S(\theta)}{d\langle S(\theta) \rangle / d\theta} = \frac{\sqrt{\langle J'^4_z \rangle - \langle J'^2_z \rangle^2}}{d\langle J'^2_z \rangle / d\theta}. \quad (27)$$

Following Ref. [15], we have computed the interferometric sensitivity of a TMSV state. To leading order in  $\bar{N}_p \gg 1$ , we find for an ideal, noiseless experiment that

$$\langle S(\theta) \rangle \approx \bar{N}_p^2 \sin^2 \theta, \quad (28)$$

$$\Delta S^2(\theta) \approx 8\bar{N}_p^4 \sin^4 \theta + \bar{N}_p^2 \sin^2 \theta \cos^2 \theta. \quad (29)$$

These expressions have the same structure as in Ref. [15], but with different numerical factors. This comes from the fact that here, the pair number is distributed according to a Bose–Einstein law of mean  $\bar{N}_p$ , whereas the pair number is fixed in Ref. [15].

The interferometric sensitivity

$$\Delta\theta \approx \left( 2 \tan^2 \theta + \frac{1}{4\bar{N}_p^2} \right)^{1/2} \quad (30)$$

is minimum at  $\theta^* = 0$ , where its value is  $\Delta\theta^* = 1/(2\bar{N}_p)$ , thus achieving the Heisenberg limit.

To determine the sensitivity in realistic conditions, we take the finite experimental resolution into account. We assume that the output signal of the interferometer is contaminated by an additive noise  $\xi$ , statistically independent of the atomic distribution. We readily find the moments of the measured signal  $\hat{J}''_z = \hat{J}'_z + \xi$  as

$$\langle \hat{J}''^2_z \rangle = \langle \hat{J}'^2_z \rangle + \langle \xi^2 \rangle, \quad (31)$$

$$\langle \hat{J}''^4_z \rangle - \langle \hat{J}''^2_z \rangle^2 = \langle \hat{J}'^4_z \rangle - \langle \hat{J}'^2_z \rangle^2 + 4\Delta\xi^2 \langle \hat{J}'^2_z \rangle + (\Delta\xi)_4. \quad (32)$$

where  $\Delta\xi^2 = \langle \xi^2 \rangle$  and  $(\Delta\xi)_4 = \langle \xi^4 \rangle - \langle \xi^2 \rangle^2$  characterize the measurement noise. The interferometric sensitivity is finally given by

$$\Delta\theta \approx \left( 2 \tan^2 \theta + \frac{1}{4\bar{N}_p^2} + \frac{\Delta\xi^2}{\bar{N}_p^2 \cos^2 \theta} + \frac{(\Delta\xi)_4}{\bar{N}_p^4 \sin^2(2\theta)} \right)^{1/2}. \quad (33)$$

For small noise levels where  $\Delta\xi^2, (\Delta\xi)_4$  are of order one and therefore small compared to  $\bar{N}_p \gg 1$ , the best sensitivity point is slightly shifted from  $\theta = 0$  to  $\theta^* \approx$

$[(\Delta\xi)_4/8]^{1/4}/\bar{N}_p$ . The best sensitivity still obeys Heisenberg scaling with  $\bar{N}_p$ , albeit with a numerical prefactor larger than the one obtained in the ideal situation. If we further assume that  $\xi$  obeys Gaussian statistics with  $\Delta\xi^2 = \sigma^2$  and  $(\Delta\xi)_4 = 3\sigma^4$ , we find

$$\Delta\theta^* \approx \frac{1}{2\bar{N}_p} \left[ 1 + 4(1 + \sqrt{6})\sigma^2 \right]^{1/2}. \quad (34)$$

Using the mean pair number  $\bar{N}_p \approx 105$  and the additive noise  $\sigma = 1.6$  as in our experiment, we obtain a phase resolution of  $\Delta\theta^* \approx 0.029$ . The standard quantum limit is  $\Delta\theta_{\text{SQL}} = 1/\sqrt{2\bar{N}_p} \approx 0.069$ , leading to a potential metrological gain  $\Delta\theta_{\text{SQL}}^2/\Delta\theta^{*2} \approx 5.8$ , *i.e.* 7.6 dB.

## VI. INTERACTING PARAMETRIC AMPLIFIER

In this paragraph we detail the dynamics of pair production and we explain the observed deviations from the predictions derived within the Bogoliubov approximation. As discussed in the main text, while one expects the increasing depletion of the pump mode  $m = 0$  to slow down the dynamics, interactions between the pump and the output modes  $m = \pm 1$  lead in fact to a counter-intuitive speed-up in our driven system.

### A. Qualitative discussion within the Bogoliubov approximation

For completeness, we recall first the main ingredients of the physics under discussion described by the generic two-mode squeezing Hamiltonian,

$$\hat{H} = \sum_{\alpha=\pm 1} V \hat{a}_\alpha^\dagger \hat{a}_\alpha + W(\hat{a}_{+1} \hat{a}_{-1} + \text{h.c.}) \quad (35)$$

with  $V, W$  real numbers. The squeezing Hamiltonian is relevant to several physical systems, for instance an ideal optical parametric amplifier, a spinor BEC in a static magnetic field, or a driven spinor BEC where the magnetic field is modulated near-resonantly around a bias value. In quantum optics, the two-mode squeezing Hamiltonian in Eq. (35) is derived from a more general Hamiltonian by making the “undepleted pump” approximation (UPA). For quantum fluids, one reaches (35) by a systematic expansion in terms of the creation and annihilation operators for the initially empty modes, restricting to second order terms (Bogoliubov approximation). In the context of spinor BECs, the diagonal term  $\propto V$  in (35) includes single-particle energy offsets and spin-conserving interactions, while the off-diagonal term  $\propto W$  describes spin-changing interactions [see Eq. (4) of the article].

The squeezing Hamiltonian is diagonalized by a Bogoliubov transformation,  $\hat{H} = E_0 + \hbar\omega_B(\hat{\alpha}^\dagger \hat{\alpha} + \hat{\beta}^\dagger \hat{\beta})$ , with  $E_0$

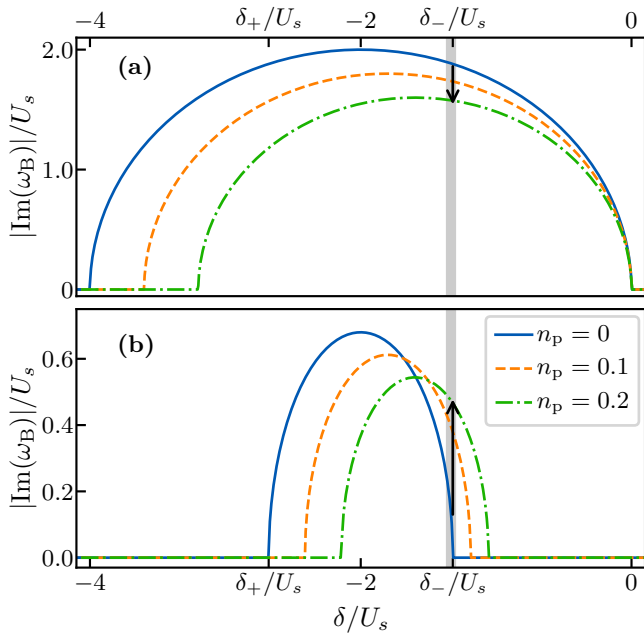

FIG. 8. **Effect of pump depletion on the pair production rate.** The rate is calculated in the Bogoliubov depleted pump approximation, where the effective interaction decreases when the mean number of pairs increases. **a.** Static case,  $\kappa = 1$ . **b.** Driven case,  $\kappa = 0.34$ . The gray vertical line indicates a particular detuning where the instability rate decreases as  $n_p$  increases in the static case, but instead increases with  $n_p$  in the driven case.

a constant and  $\hat{\alpha}, \hat{\beta}$  the Bogoliubov modes annihilation operators. The Bogoliubov energy is given by

$$\hbar\omega_B = \sqrt{\lambda_+ \lambda_-} \quad (36)$$

with  $\lambda_{\pm} = V \pm W$ . A dynamical instability arises when  $\omega_B$  is purely imaginary, *i.e.*  $|V| < |W|$ . This regime corresponds to an exponential production of pairs from the vacuum state at an initial rate  $|\omega_B|$ .

In the UPA or Bogoliubov approximation, both static and driven spinor BECs can be described by  $V = U_s + \hbar\delta/2$  and  $W = \kappa U_s > 0$ , so that  $\lambda_{\pm} = \hbar\delta/2 + U_s(1 \pm \kappa)$ . The region of instability occurs for negative detunings  $\delta_+ \leq \delta \leq \delta_-$ , with  $\delta_{\pm} = -2U_s(1 \pm \kappa)$  [16]. Here  $U_s$  is the bare spin-dependent interaction energy. In the static case,  $\hbar\delta/2$  corresponds to the quadratic Zeeman energy and  $\kappa = 1$ : spin-conserving and spin-mixing interactions have the same strength. In the driven case, the detuning  $\delta$  and the renormalization factor  $\kappa < 1$  characterize the

secular dynamics, much slower than the drive frequency (see main text and [16]). Since  $\kappa < 1$ , the effective spin-mixing interactions are weaker than the spin-conserving ones.

In order to qualitatively understand the role of saturation and interaction effects beyond the UPA, we propose a mean-field extension of the UPA where  $\hat{a}_0 \approx \sqrt{N(1 - 2\bar{n}_p)}$ , with  $\bar{n}_p = \langle \hat{N}_p \rangle / N$  the normalized average number of  $\pm 1$  pairs. This “depleted pump approximation” amounts to a renormalization of  $U_s$  to  $\tilde{U}_s = U_s(1 - 2\bar{n}_p)$ . To understand how this impacts the dynamics, we plot in Fig. 8 the pair production rate  $|\omega_B|$  versus detuning for several depletion levels. For the chosen detuning indicated by the gray line, the static and driven systems behave completely differently, with a rate decreasing with  $\bar{n}_p$  in the first case, but increasing with  $\bar{n}_p$  in the second.

The difference can be traced back to the different roles of spin-conserving and spin-mixing interactions in determining the Bogoliubov rate  $|\omega_B| = \sqrt{|\lambda_+ \lambda_-|}$ . As a function of  $\delta$ , the rate looks like an inverted parabola centered around  $\hbar\delta = -2\tilde{U}_s$  (determined by the spin-conserving interactions) and with a maximal value  $\kappa\tilde{U}_s$  (determined by the spin-mixing interactions). As  $\tilde{U}_s$  decreases ( $\bar{n}_p$  increases), the maximum is pushed towards positive detunings and its value decreases. In the static case, the two phenomena happen exactly at the same rate and the dynamics always becomes slower with increasing depletion. In the driven case, the shift of the position of the maximum is larger than the decrease of the peak value, due to the renormalization factor  $\kappa$ . As a result, one can find a range of detuning close to the upper edge  $\delta_-$  where the derivative  $\partial|\omega_B|/\partial\tilde{U}_s$  becomes negative, implying an “amplification” of pair production with depletion in comparison with the UPA prediction.

## B. Numerical resolution

In Fig. 9, we compare the predictions derived from the Bogoliubov Hamiltonian (35) with those obtained numerically without approximation, beyond those leading to the secular Hamiltonian [Eq. (6) in the main text]. We introduce the variables  $\delta' = \delta + 2U_s/\hbar$  and  $U' = \kappa U_s$ . In Fig. 9a, we plot the maximal number of pairs produced over a time  $t = 5\hbar/U'$  versus  $\delta'$ . In Fig. 9b, we show the time evolution of  $N_p$  for  $\hbar\delta' = 2U'$ , on the upper boundary of the instability domain. The competition between the depletion of the pump and the pump-output interaction explains qualitatively all observed features.

[1] The effective numerical aperture is slightly reduced from the numerical aperture of the front-end microscope objective  $\approx 0.33$  due to the spatial mask blocking the back-ground light.

[2] T. W. Hodapp, C. Gerz, C. Furtlehner, C. I. Westbrook, W. D. Phillips, and J. Dalibard, “Three-dimensional spatial diffusion in optical molasses,” *Applied Physics B* **60**, 135–143 (1995)

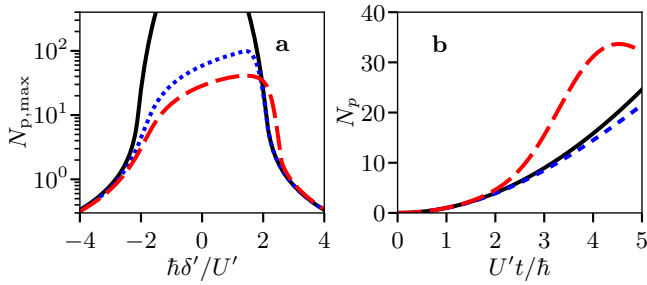

FIG. 9. **a.** Average number of pairs  $N_p$  produced after an evolution time  $t = 5\hbar/U'$ , versus  $\hbar\delta'/U'$ . **b.** Evolution of  $N_p$  for  $\hbar\delta' = 2U'$ . The solid black line represents the result obtained with the Bogoliubov Hamiltonian. The blue dotted line shows the result obtained with the full secular Hamiltonian for static spin-mixing ( $\kappa = 1$ ). Because of the pump-output interaction, the resonance is shifted to the right. Close to the upper boundary of the instability region  $\hbar\delta' = 2U'$ , this shift counteracts the depletion, and the agreement with the Bogoliubov approximation is very good. The red dashed line shows the result obtained from the full secular Hamiltonian in the driven spin-mixing case ( $\kappa = 0.34$ ), where the pump-output interaction is stronger than the exchange interaction. Close to the boundary  $\hbar\delta' = 2U'$ , the pair production rate is larger than the Bogoliubov prediction. Here  $N = 300$ .

[3] C. F. Ockeloen, A. F. Tauschinsky, R. J. C. Spreeuw, and S. Whitlock, “Detection of small atom numbers through image processing,” *Phys. Rev. A* **82**, 061606 (Dec 2010),

[4] Max F Riedel, Pascal Böhi, Yun Li, Theodor W Hänsch, Alice Sinatra, and Philipp Treutlein, “Atom-chip-based generation of entanglement for quantum metrology,” *Nature* **464**, 1170–1173 (2010)

[5] Géza Tóth, Christian Knapp, Otfried Gühne, and Hans J. Briegel, “Optimal spin squeezing inequalities detect bound entanglement in spin models,” *Phys. Rev. Lett.* **99**, 250405 (Dec 2007),

[6] Giuseppe Vitagliano, Iagoba Apellaniz, Iñigo L. Egusquiza, and Géza Tóth, “Spin squeezing and entanglement for an arbitrary spin,” *Phys. Rev. A* **89**, 032307 (Mar 2014),

[7] Bernd Lücke, Jan Peise, Giuseppe Vitagliano, Jan Arlt, Luis Santos, Géza Tóth, and Carsten Klempt, “Detecting multiparticle entanglement of Dicke states,” *Phys. Rev. Lett.* **112**, 155304 (Apr 2014)

[8] J. K. Korbicz, J. I. Cirac, and M. Lewenstein, “Spin squeezing inequalities and entanglement of  $n$  qubit states,” *Phys. Rev. Lett.* **95**, 120502 (Sep 2005),

[9] J. K. Korbicz, J. I. Cirac, and M. Lewenstein, “Erratum: Spin squeezing inequalities and entanglement of  $n$  qubit states [phys. rev. lett. 95, 120502 (2005)],” *Phys. Rev. Lett.* **95**, 259901 (Dec 2005),

[10] Xin-Yu Luo, Yi-Quan Zou, Ling-Na Wu, Qi Liu, Ming-Fei Han, Meng Khoon Tey, and Li You, “Deterministic entanglement generation from driving through quantum phase transitions,” *Science* **355**, 620–623 (2017), ISSN 0036-8075,

[11] W. Muessel, H. Strobel, D. Linnemann, D. B. Hume, and M. K. Oberthaler, “Scalable spin squeezing for quantum-enhanced magnetometry with Bose-Einstein

condensates,” *Phys. Rev. Lett.* **113**, 103004 (Sep 2014),

[12] Eva M. Bookjans, Christopher D. Hamley, and Michael S. Chapman, “Strong quantum spin correlations observed in atomic spin mixing,” *Phys. Rev. Lett.* **107**, 210406 (Nov 2011),

[13] M. J. Holland and K. Burnett, “Interferometric detection of optical phase shifts at the Heisenberg limit,” *Phys. Rev. Lett.* **71**, 1355 (1993)

[14] P. Bouyer and M. A. Kasevich, “Heisenberg-limited spectroscopy with degenerate Bose-Einstein gases,” *Phys. Rev. A* **56**, R1083 (Aug. 1997)

[15] Taesoo Kim, Olivier Pfister, Murray J. Holland, Jaewoo Noh, and John L. Hall, “Influence of decorrelation on heisenberg-limited interferometry with quantum correlated photons,” *Phys. Rev. A* **57**, 4004–4013 (May 1998),

[16] Bertrand Evrard, An Qu, Karina Jiménez-García, Jean Dalibard, and Fabrice Gerbier, “Relaxation and hysteresis near shapiro resonances in a driven spinor condensate,” *Phys. Rev. A* **100**, 023604 (Aug 2019),
